# Supplementary material for: SPC-NeRF: Spatial Predictive Compression for Voxel Based Radiance Field
Source: arXiv:2402.16366 source file (2024-02-26)
Supplement: Supplementary file 1 [file X_suppl.tex]

\clearpage
\setcounter{page}{1}
\maketitlesupplementary

\setcounter{section}{0}
\section{Implimentation Details}
We follow the pipeline and the training configuration in DVGO\footnote{\url{https://github.com/sunset1995/DirectVoxGO}} to generate the uncompressed model. In our finetuning process, we set the initial learning rate 0.1 for both the density grid and the feature grid, and learning rate 1e-3 for the shallow MLP. The two finetune stages take 8000 and 4000 iterations, respectively, with 8192 rays per iteration. Besides, we adjust the $\lambda$ values of the high-quality configuration to obtain similar rendering quality to VQRF in table~\ref{main performance}. Specifically, the $\lambda$s are set to 1e-4 for Synthetic-NeRF and Synthetic-NSVF, and 4e-4 for the other two datasets. We then quadruple the $\lambda$s to obtain the low-quality configuration.

For the RD curves in Fig.~\ref{overall perfomance} and Fig.~\ref{scene-rd-curve}, each time we increase the $\lambda$ by a factor of 2 in our methods. The $\lambda$ ranges from 5e-5 to 8e-4 for the base configuration and from 1e-4 to 3.2e-3 for the HR configuration. In order to generate the RD curves for VQRF~\footnote{\url{https://github.com/AlgoHunt/VQRF}}, we first range the pruning quantile from 1e-3 to 2e-2 and the keeping quantile from 0.2 to 0.6 to obtain all test points. Then we calculate an upper convex hull of these points because the test points are not monotonic.

\section{Detailed Results}
We show the per-scene results of our method in the 4 datasets mentioned in the main paper: Synthetic-NeRF in Table~\ref{syn_base} and Table \ref{syn_hr}; Synthetic-NSVF in Table~\ref{nsvf_base} and Table~\ref{nsvf_hr}; Blended-MVS in Table~\ref{mvs_base} and Table~\ref{mvs_hr}; Tanks \& Temples in Table~\ref{tnt} and Table~\ref{tnt_hr}. Both PSNR and the perceptual results indicate that our method can achieve a compression of over 100 times with negligible degradation in rendering quality. By adjusting the trade-off coefficient $\lambda$, our method can further increase the compression ratio while keeping the distortion within an acceptable range, validating the effectiveness and versatility of our method.

\begin{figure*}[htp]
\centering
\includegraphics[width=0.85\textwidth]{CVPR SM_subjective_syn.pdf} % Reduce the figure size so that it is slightly narrower than the column.
\caption{We randomly show rendered pictures of one view for each scene in the Synthetic NeRF dataset. All pictures above are lossless compressed.}
\label{smsub1}
\end{figure*}

\begin{figure*}[htp]
\centering
\includegraphics[width=0.85\textwidth]{CVPR SM_subjective_nsvf.pdf} % Reduce the figure size so that it is slightly narrower than the column.
\caption{We randomly show rendered pictures of one view for each scene in the Synthetic NSVF dataset. All pictures above are lossless compressed.}
\label{smsub2}
\end{figure*}

\begin{figure*}[htp]
\centering
\includegraphics[width=0.85\textwidth]{CVPR SM_subjective_mvs.pdf} % Reduce the figure size so that it is slightly narrower than the column.
\caption{We randomly show rendered pictures of one view for each scene in the BlendedMVS dataset. All pictures above are lossless compressed.}
\label{smsub3}
\end{figure*}

\begin{figure*}[htp]
\centering
\includegraphics[width=0.85\textwidth]{CVPR SM_subjective_tnt.pdf} % Reduce the figure size so that it is slightly narrower than the column.
\caption{We randomly show rendered pictures of one view for each scene in the Tanks \& Temples dataset. All pictures above are lossless compressed.}
\label{smsub4}
\end{figure*}

\section{More Subjective Results}
We demonstrate the degradation of subjective quality as we increase x in the base configuration, i.e. with a voxel resolution of $160^3$. We show the rendered pictures in Fig~\ref{smsub1} to Fig~\ref{smsub4}. All pictures we show in these figures are lossless compressed. The results indicate that the degradation of subjective quality is still marginal even when the compression ratio reaches nearly 200 times.

\begin{table*}[h]
    \centering
    \setlength{\tabcolsep}{5pt} % Adjust horizontal spacing
    \linespread{1.2} \selectfont
    \small
    \begin{tabular}{ccccccccccc}
        \toprule
        \multicolumn{11}{c}{Synthetic NeRF} \\
        ~ & Method & chair & drums & ficus & hotdog & lego & materials & mic & ship & Average \\ 
        \midrule \midrule
        \multirow{8}{*}{SIZE~(MB)$\downarrow$} & DVGO & 106.5  & 95.8  & 109.9  & 133.8  & 124.5  & 176.1  & 49.9  & 103.4  & 112.5  \\ 
        ~ & Ours$_{\lambda=5e-5}$ & 0.928  & 0.891  & 0.963  & 1.083  & 1.276  & 2.785  & 0.320  & 1.946  & 1.274  \\ 
        ~ & Ours$_{\lambda=1e-4}$ & 0.833  & 0.808  & 0.854  & 1.006  & 1.144  & 2.533  & 0.289  & 1.739  & 1.151  \\ 
        ~ & Ours$_{\lambda=2e-4}$ & 0.699  & 0.680  & 0.703  & 0.828  & 0.942  & 2.096  & 0.245  & 1.413  & 0.951  \\ 
        ~ & Ours$_{\lambda=4e-4}$ & 0.602  & 0.588  & 0.603  & 0.737  & 0.815  & 1.798  & 0.217  & 1.193  & 0.819  \\ 
        ~ & Ours$_{\lambda=8e-4}$ & 0.525  & 0.513  & 0.528  & 0.669  & 0.721  & 1.558  & 0.195  & 1.027  & 0.717  \\ 
        ~ & Ours$_{\lambda=1.6e-3}$ & 0.463  & 0.454  & 0.476  & 0.622  & 0.656  & 1.377  & 0.178  & 0.913  & 0.642  \\ 
        ~ & Ours$_{\lambda=6.4e-3}$ & 0.398  & 0.387  & 0.423  & 0.575  & 0.584  & 1.168  & 0.158  & 0.788  & 0.560  \\ \midrule
        \multirow{8}{*}{PSNR~(dB)$\uparrow$} & DVGO & 34.09  & 25.47  & 32.71  & 36.67  & 34.59  & 29.52  & 33.14  & 29.12  & 31.91  \\ 
        ~ & Ours$_{\lambda=5e-5}$ & 33.91  & 25.44  & 32.63  & 36.47  & 34.34  & 29.46  & 33.06  & 29.21  & 31.82  \\ 
        ~ & Ours$_{\lambda=1e-4}$ & 33.81  & 25.43  & 32.61  & 36.33  & 34.25  & 29.47  & 32.91  & 29.19  & 31.75  \\ 
        ~ & Ours$_{\lambda=2e-4}$ & 33.61  & 25.41  & 32.57  & 36.22  & 34.04  & 29.43  & 32.80  & 29.15  & 31.65  \\ 
        ~ & Ours$_{\lambda=4e-4}$ & 33.32  & 25.37  & 32.51  & 36.01  & 33.77  & 29.39  & 32.57  & 29.08  & 31.50  \\ 
        ~ & Ours$_{\lambda=8e-4}$ & 32.90  & 25.30  & 32.40  & 35.71  & 33.38  & 29.32  & 32.23  & 28.95  & 31.27  \\ 
        ~ & Ours$_{\lambda=1.6e-3}$ & 32.38  & 25.21  & 32.18  & 35.29  & 32.93  & 29.21  & 31.77  & 28.71  & 30.96  \\ 
        ~ & Ours$_{\lambda=6.4e-3}$ & 31.10  & 24.86  & 31.58  & 34.43  & 31.70  & 28.80  & 30.80  & 28.13  & 30.18  \\ \midrule
        \multirow{8}{*}{SSIM$\uparrow$} & DVGO & 0.976  & 0.930  & 0.978  & 0.980  & 0.976  & 0.950  & 0.983  & 0.878  & 0.956  \\ 
        ~ & Ours$_{\lambda=5e-5}$ & 0.975  & 0.929  & 0.977  & 0.978  & 0.974  & 0.948  & 0.981  & 0.878  & 0.955  \\ 
        ~ & Ours$_{\lambda=1e-4}$ & 0.974  & 0.928  & 0.977  & 0.977  & 0.973  & 0.948  & 0.981  & 0.877  & 0.954  \\ 
        ~ & Ours$_{\lambda=2e-4}$ & 0.972  & 0.928  & 0.977  & 0.976  & 0.972  & 0.947  & 0.980  & 0.876  & 0.953  \\ 
        ~ & Ours$_{\lambda=4e-4}$ & 0.970  & 0.927  & 0.976  & 0.974  & 0.970  & 0.947  & 0.978  & 0.874  & 0.952  \\ 
        ~ & Ours$_{\lambda=8e-4}$ & 0.967  & 0.926  & 0.975  & 0.972  & 0.966  & 0.945  & 0.976  & 0.870  & 0.950  \\ 
        ~ & Ours$_{\lambda=1.6e-3}$ & 0.962  & 0.924  & 0.974  & 0.969  & 0.962  & 0.944  & 0.973  & 0.865  & 0.947  \\ 
        ~ & Ours$_{\lambda=6.4e-3}$ & 0.949  & 0.918  & 0.970  & 0.962  & 0.950  & 0.937  & 0.965  & 0.853  & 0.938  \\ \midrule
        \multirow{5}{*}{LPIPS$_{ALEX}\downarrow$} & DVGO & 0.027  & 0.078  & 0.025  & 0.034  & 0.027  & 0.059  & 0.018  & 0.160  & 0.054  \\ 
        ~ & Ours$_{\lambda=1e-4}$ & 0.032  & 0.081  & 0.027  & 0.047  & 0.031  & 0.064  & 0.024  & 0.164  & 0.059  \\ 
        ~ & Ours$_{\lambda=4e-4}$ & 0.036  & 0.083  & 0.028  & 0.053  & 0.037  & 0.067  & 0.028  & 0.170  & 0.063  \\ 
        ~ & Ours$_{\lambda=1.6e-3}$ & 0.045  & 0.087  & 0.031  & 0.062  & 0.047  & 0.072  & 0.035  & 0.181  & 0.070  \\ 
        ~ & Ours$_{\lambda=6.4e-3}$ & 0.058  & 0.094  & 0.035  & 0.073  & 0.060  & 0.079  & 0.044  & 0.197  & 0.080  \\ \midrule
        \multirow{5}{*}{LPIPS$_{VGG}\downarrow$} & DVGO & 0.017  & 0.060  & 0.015  & 0.018  & 0.013  & 0.027  & 0.014  & 0.117  & 0.035  \\ 
        ~ & Ours$_{\lambda=1e-4}$ & 0.018  & 0.061  & 0.016  & 0.022  & 0.015  & 0.030  & 0.017  & 0.120  & 0.037  \\ 
        ~ & Ours$_{\lambda=4e-4}$ & 0.023  & 0.063  & 0.017  & 0.026  & 0.017  & 0.032  & 0.019  & 0.127  & 0.041  \\ 
        ~ & Ours$_{\lambda=1.6e-3}$ & 0.032  & 0.068  & 0.019  & 0.033  & 0.021  & 0.035  & 0.026  & 0.138  & 0.047  \\ 
        ~ & Ours$_{\lambda=6.4e-3}$ & 0.046  & 0.077  & 0.022  & 0.041  & 0.028  & 0.042  & 0.036  & 0.153  & 0.056 \\ 
        \bottomrule
    \end{tabular}
    \caption{Per scene results on Synthetic NeRF dataset with the voxel resolution set to $160^3$. Note we do not evaluate LPIPS for all test configurations.}
\label{syn_base}
\end{table*}

\begin{table*}[h]
    \centering
    \setlength{\tabcolsep}{5pt} % Adjust horizontal spacing
    \linespread{1.2} \selectfont
    \small
    \begin{tabular}{ccccccccccc}
        \toprule
        \multicolumn{11}{c}{Synthetic NeRF~(HR)} \\
        ~ & Method & chair & drums & ficus & hotdog & lego & materials & mic & ship & Average \\ 
        \midrule \midrule
        \multirow{8}{*}{SIZE~(MB)$\downarrow$} & DVGO & 384.8  & 326.9  & 408.5  & 487.1  & 472.7  & 670.7  & 152.7  & 374.8  & 409.8  \\ 
        ~ & Ours$_{\lambda=1e-4}$ & 2.541  & 2.458  & 2.344  & 3.126  & 3.758  & 8.588  & 0.845  & 6.505  & 3.771  \\ 
        ~ & Ours$_{\lambda=2e-4}$ & 2.206  & 2.141  & 2.037  & 2.740  & 3.281  & 7.557  & 0.736  & 5.603  & 3.288  \\ 
        ~ & Ours$_{\lambda=4e-4}$ & 1.904  & 1.852  & 1.772  & 2.421  & 2.873  & 6.596  & 0.643  & 4.746  & 2.851  \\ 
        ~ & Ours$_{\lambda=8e-4}$ & 1.653  & 1.610  & 1.558  & 2.170  & 2.551  & 5.759  & 0.569  & 4.027  & 2.487  \\ 
        ~ & Ours$_{\lambda=1.6e-3}$ & 1.454  & 1.417  & 1.403  & 1.985  & 2.315  & 5.087  & 0.511  & 3.482  & 2.207  \\ 
        ~ & Ours$_{\lambda=3.2e-3}$ & 1.329  & 1.285  & 1.291  & 1.857  & 2.150  & 4.582  & 0.470  & 3.112  & 2.009  \\ 
        ~ & Ours$_{\lambda=6.4e-3}$ & 1.233  & 1.186  & 1.223  & 1.775  & 2.040  & 4.232  & 0.442  & 2.867  & 1.875  \\ \midrule
        \multirow{8}{*}{PSNR~(dB)$\uparrow$} & DVGO & 35.35  & 25.82  & 33.64  & 37.06  & 35.90  & 29.58  & 34.72  & 30.05  & 32.77  \\ 
        ~ & Ours$_{\lambda=1e-4}$ & 35.18  & 25.79  & 33.64  & 36.91  & 35.68  & 29.58  & 34.57  & 30.27  & 32.70  \\ 
        ~ & Ours$_{\lambda=2e-4}$ & 35.09  & 25.78  & 33.64  & 36.84  & 35.60  & 29.58  & 34.50  & 30.26  & 32.66  \\ 
        ~ & Ours$_{\lambda=4e-4}$ & 34.92  & 25.77  & 33.64  & 36.73  & 35.48  & 29.57  & 34.36  & 30.24  & 32.59  \\ 
        ~ & Ours$_{\lambda=8e-4}$ & 34.65  & 25.74  & 33.60  & 36.58  & 35.30  & 29.56  & 34.13  & 30.19  & 32.47  \\ 
        ~ & Ours$_{\lambda=1.6e-3}$ & 34.26  & 25.69  & 33.50  & 36.34  & 35.02  & 29.52  & 33.76  & 30.09  & 32.27  \\ 
        ~ & Ours$_{\lambda=3.2e-3}$ & 33.74  & 25.60  & 33.39  & 36.05  & 34.62  & 29.48  & 33.26  & 29.93  & 32.01  \\ 
        ~ & Ours$_{\lambda=6.4e-3}$ & 33.16  & 25.50  & 33.16  & 35.67  & 34.16  & 29.36  & 32.69  & 29.70  & 31.68  \\ \midrule
        \multirow{8}{*}{SSIM$\uparrow$} & DVGO & 0.983  & 0.936  & 0.982  & 0.982  & 0.981  & 0.950  & 0.988  & 0.893  & 0.962  \\ 
        ~ & Ours$_{\lambda=1e-4}$ & 0.982  & 0.934  & 0.981  & 0.980  & 0.979  & 0.949  & 0.987  & 0.892  & 0.961  \\ 
        ~ & Ours$_{\lambda=2e-4}$ & 0.981  & 0.934  & 0.981  & 0.979  & 0.979  & 0.948  & 0.987  & 0.892  & 0.960  \\ 
        ~ & Ours$_{\lambda=4e-4}$ & 0.981  & 0.934  & 0.981  & 0.978  & 0.978  & 0.948  & 0.986  & 0.892  & 0.960  \\ 
        ~ & Ours$_{\lambda=8e-4}$ & 0.979  & 0.933  & 0.981  & 0.977  & 0.977  & 0.948  & 0.985  & 0.890  & 0.959  \\ 
        ~ & Ours$_{\lambda=1.6e-3}$ & 0.977  & 0.933  & 0.980  & 0.976  & 0.975  & 0.947  & 0.983  & 0.888  & 0.957  \\ 
        ~ & Ours$_{\lambda=3.2e-3}$ & 0.973  & 0.931  & 0.979  & 0.973  & 0.972  & 0.946  & 0.981  & 0.884  & 0.955  \\ 
        ~ & Ours$_{\lambda=6.4e-3}$ & 0.969  & 0.929  & 0.978  & 0.971  & 0.969  & 0.944  & 0.978  & 0.880  & 0.952  \\ \midrule
        \multirow{5}{*}{LPIPS$_{ALEX}\downarrow$} & DVGO & 0.019  & 0.068  & 0.020  & 0.030  & 0.020  & 0.056  & 0.012  & 0.139  & 0.046  \\ 
        ~ & Ours$_{\lambda=1e-4}$ & 0.023  & 0.071  & 0.021  & 0.042  & 0.022  & 0.059  & 0.016  & 0.140  & 0.049  \\ 
        ~ & Ours$_{\lambda=4e-4}$ & 0.024  & 0.072  & 0.022  & 0.047  & 0.024  & 0.060  & 0.018  & 0.144  & 0.051  \\ 
        ~ & Ours$_{\lambda=1.6e-3}$ & 0.029  & 0.074  & 0.023  & 0.053  & 0.028  & 0.063  & 0.023  & 0.151  & 0.055  \\ 
        ~ & Ours$_{\lambda=6.4e-3}$ & 0.037  & 0.079  & 0.026  & 0.061  & 0.036  & 0.069  & 0.029  & 0.161  & 0.062  \\ \midrule
        \multirow{5}{*}{LPIPS$_{VGG}\downarrow$} & DVGO & 0.010  & 0.050  & 0.013  & 0.014  & 0.009  & 0.024  & 0.008  & 0.090  & 0.027  \\ 
        ~ & Ours$_{\lambda=1e-4}$ & 0.011  & 0.051  & 0.013  & 0.017  & 0.010  & 0.026  & 0.009  & 0.090  & 0.029  \\ 
        ~ & Ours$_{\lambda=4e-4}$ & 0.012  & 0.052  & 0.013  & 0.019  & 0.010  & 0.027  & 0.011  & 0.094  & 0.030  \\ 
        ~ & Ours$_{\lambda=1.6e-3}$ & 0.015  & 0.054  & 0.014  & 0.023  & 0.012  & 0.028  & 0.014  & 0.102  & 0.033  \\ 
        ~ & Ours$_{\lambda=6.4e-3}$ & 0.022  & 0.059  & 0.016  & 0.028  & 0.015  & 0.032  & 0.020  & 0.113  & 0.038 \\ 
        \bottomrule
    \end{tabular}
    \caption{Per scene results on Synthetic NeRF dataset with the voxel resolution set to $256^3$~(HR). Note we do not evaluate LPIPS for all test configurations.}
\label{syn_hr}
\end{table*}

\begin{table*}[h]
    \centering
    \setlength{\tabcolsep}{5pt} % Adjust horizontal spacing
    \linespread{1.2} \selectfont
    \small
    \begin{tabular}{ccccccccccc}
        \toprule
        \multicolumn{11}{c}{Synthetic NSVF} \\
        ~ & Method & Bike & Lifestyle & Palace & Robot & Spaceship & Steamtrain & Toad & Wineholder & Average \\ 
        \midrule \midrule
        \multirow{5}{*}{SIZE~(MB)$\downarrow$} & DVGO & 114.9  & 103.7  & 109.3  & 102.2  & 132.3  & 156.2  & 133.4  & 106.4  & 119.8  \\ 
        ~ & Ours$_{\lambda=1e-4}$ & 0.837  & 0.818  & 1.378  & 0.863  & 1.403  & 1.629  & 0.730  & 0.748  & 1.051  \\ 
        ~ & Ours$_{\lambda=4e-4}$ & 0.580  & 0.575  & 0.965  & 0.615  & 0.979  & 1.182  & 0.529  & 0.532  & 0.745  \\ 
        ~ & Ours$_{\lambda=1.6e-3}$ & 0.467  & 0.466  & 0.758  & 0.482  & 0.781  & 0.956  & 0.404  & 0.418  & 0.591  \\ 
        ~ & Ours$_{\lambda=6.4e-3}$ & 0.417  & 0.417  & 0.664  & 0.414  & 0.689  & 0.845  & 0.342  & 0.367  & 0.519  \\ \midrule
        \multirow{5}{*}{PSNR~(dB)$\uparrow$} & DVGO & 38.17  & 33.74  & 34.43  & 36.39  & 37.52  & 35.42  & 32.98  & 30.29  & 34.87  \\ 
        ~ & Ours$_{\lambda=1e-4}$ & 37.50  & 33.49  & 34.21  & 36.23  & 37.43  & 35.32  & 32.45  & 30.15  & 34.60  \\ 
        ~ & Ours$_{\lambda=4e-4}$ & 37.25  & 33.26  & 33.89  & 35.76  & 37.29  & 35.25  & 31.74  & 29.99  & 34.30  \\ 
        ~ & Ours$_{\lambda=1.6e-3}$ & 36.58  & 32.70  & 33.14  & 34.86  & 36.82  & 35.02  & 30.25  & 29.66  & 33.63  \\ 
        ~ & Ours$_{\lambda=6.4e-3}$ & 35.55  & 31.93  & 32.06  & 33.44  & 36.00  & 34.54  & 28.56  & 29.13  & 32.65  \\ \midrule
        \multirow{5}{*}{SSIM$\uparrow$} & DVGO & 0.991  & 0.965  & 0.962  & 0.992  & 0.987  & 0.987  & 0.965  & 0.950  & 0.975  \\ 
        ~ & Ours$_{\lambda=1e-4}$ & 0.990  & 0.962  & 0.959  & 0.991  & 0.987  & 0.986  & 0.960  & 0.948  & 0.973  \\ 
        ~ & Ours$_{\lambda=4e-4}$ & 0.989  & 0.959  & 0.955  & 0.990  & 0.986  & 0.985  & 0.951  & 0.945  & 0.970  \\ 
        ~ & Ours$_{\lambda=1.6e-3}$ & 0.987  & 0.953  & 0.945  & 0.988  & 0.985  & 0.984  & 0.929  & 0.940  & 0.964  \\ 
        ~ & Ours$_{\lambda=6.4e-3}$ & 0.984  & 0.946  & 0.929  & 0.984  & 0.982  & 0.981  & 0.896  & 0.933  & 0.955  \\ \midrule
        \multirow{5}{*}{LPIPS$_{ALEX}\downarrow$} & DVGO & 0.011  & 0.053  & 0.043  & 0.013  & 0.020  & 0.022  & 0.046  & 0.054  & 0.033  \\ 
        ~ & Ours$_{\lambda=1e-4}$ & 0.014  & 0.060  & 0.046  & 0.014  & 0.021  & 0.026  & 0.053  & 0.057  & 0.036  \\ 
        ~ & Ours$_{\lambda=4e-4}$ & 0.015  & 0.065  & 0.052  & 0.015  & 0.022  & 0.027  & 0.066  & 0.059  & 0.040  \\ 
        ~ & Ours$_{\lambda=1.6e-3}$ & 0.018  & 0.072  & 0.062  & 0.018  & 0.023  & 0.030  & 0.088  & 0.064  & 0.047  \\ 
        ~ & Ours$_{\lambda=6.4e-3}$ & 0.021  & 0.079  & 0.076  & 0.022  & 0.026  & 0.033  & 0.114  & 0.071  & 0.055  \\ \midrule
        \multirow{5}{*}{LPIPS$_{VGG}\downarrow$} & DVGO & 0.004  & 0.026  & 0.027  & 0.005  & 0.010  & 0.011  & 0.030  & 0.036  & 0.019  \\ 
        ~ & Ours$_{\lambda=1e-4}$ & 0.005  & 0.029  & 0.028  & 0.005  & 0.010  & 0.012  & 0.034  & 0.037  & 0.020  \\ 
        ~ & Ours$_{\lambda=4e-4}$ & 0.005  & 0.033  & 0.032  & 0.006  & 0.011  & 0.012  & 0.043  & 0.039  & 0.023  \\ 
        ~ & Ours$_{\lambda=1.6e-3}$ & 0.006  & 0.038  & 0.039  & 0.008  & 0.012  & 0.013  & 0.061  & 0.045  & 0.028  \\ 
        ~ & Ours$_{\lambda=6.4e-3}$ & 0.008  & 0.044  & 0.049  & 0.011  & 0.014  & 0.015  & 0.086  & 0.051  & 0.035 \\ 
        \bottomrule
    \end{tabular}
    \caption{Per scene results on Synthetic NSVF dataset with the voxel resolution set to $160^3$.}
\label{nsvf_base}
\end{table*}

\begin{table*}[h]
    \centering
    \setlength{\tabcolsep}{5pt} % Adjust horizontal spacing
    \linespread{1.2} \selectfont
    \small
    \begin{tabular}{ccccccccccc}
        \toprule
        \multicolumn{11}{c}{Synthetic NSVF~(HR)} \\
        ~ & Method & Bike & Lifestyle & Palace & Robot & Spaceship & Steamtrain & Toad & Wineholder & Average \\ 
        \midrule \midrule
        \multirow{5}{*}{SIZE~(MB)$\downarrow$} & DVGO & 424.7  & 371.7  & 417.5  & 382.5  & 509.0  & 622.6  & 496.9  & 381.8  & 450.8  \\ 
        ~ & Ours$_{\lambda=1e-4}$ & 2.586  & 2.671  & 4.547  & 2.436  & 4.459  & 5.154  & 2.500  & 2.391  & 3.343  \\ 
        ~ & Ours$_{\lambda=4e-4}$ & 1.949  & 2.044  & 3.432  & 1.838  & 3.387  & 3.987  & 1.862  & 1.773  & 2.534  \\ 
        ~ & Ours$_{\lambda=1.6e-3}$ & 1.547  & 1.629  & 2.658  & 1.446  & 2.669  & 3.208  & 1.418  & 1.357  & 1.992  \\ 
        ~ & Ours$_{\lambda=6.4e-3}$ & 1.354  & 1.428  & 2.273  & 1.247  & 2.300  & 2.804  & 1.191  & 1.147  & 1.718  \\ \midrule
        \multirow{5}{*}{PSNR~(dB)$\uparrow$} & DVGO & 39.10  & 34.60  & 36.83  & 38.37  & 38.07  & 36.20  & 34.97  & 31.34  & 36.18  \\ 
        ~ & Ours$_{\lambda=1e-4}$ & 38.76  & 34.56  & 36.73  & 38.31  & 38.04  & 36.10  & 34.75  & 31.31  & 36.07  \\ 
        ~ & Ours$_{\lambda=4e-4}$ & 38.64  & 34.43  & 36.49  & 38.12  & 38.00  & 36.09  & 34.16  & 31.23  & 35.90  \\ 
        ~ & Ours$_{\lambda=1.6e-3}$ & 38.30  & 34.12  & 35.96  & 37.60  & 37.82  & 36.03  & 32.92  & 30.99  & 35.47  \\ 
        ~ & Ours$_{\lambda=6.4e-3}$ & 37.60  & 33.53  & 34.99  & 36.58  & 37.34  & 35.82  & 31.14  & 30.53  & 34.69  \\ \midrule
        \multirow{5}{*}{SSIM$\uparrow$} & DVGO & 0.993  & 0.970  & 0.976  & 0.994  & 0.988  & 0.988  & 0.978  & 0.961  & 0.981  \\ 
        ~ & Ours$_{\lambda=1e-4}$ & 0.992  & 0.969  & 0.975  & 0.994  & 0.987  & 0.987  & 0.976  & 0.960  & 0.980  \\ 
        ~ & Ours$_{\lambda=4e-4}$ & 0.992  & 0.967  & 0.973  & 0.994  & 0.987  & 0.987  & 0.972  & 0.959  & 0.979  \\ 
        ~ & Ours$_{\lambda=1.6e-3}$ & 0.991  & 0.963  & 0.969  & 0.993  & 0.987  & 0.987  & 0.962  & 0.956  & 0.976  \\ 
        ~ & Ours$_{\lambda=6.4e-3}$ & 0.989  & 0.958  & 0.960  & 0.991  & 0.986  & 0.985  & 0.943  & 0.949  & 0.970  \\ \midrule
        \multirow{5}{*}{LPIPS$_{ALEX}\downarrow$} & DVGO & 0.009  & 0.043  & 0.026  & 0.010  & 0.019  & 0.020  & 0.030  & 0.043  & 0.025  \\ 
        ~ & Ours$_{\lambda=1e-4}$ & 0.011  & 0.046  & 0.027  & 0.010  & 0.020  & 0.023  & 0.032  & 0.044  & 0.027  \\ 
        ~ & Ours$_{\lambda=4e-4}$ & 0.012  & 0.050  & 0.030  & 0.011  & 0.020  & 0.024  & 0.038  & 0.046  & 0.029  \\ 
        ~ & Ours$_{\lambda=1.6e-3}$ & 0.013  & 0.056  & 0.035  & 0.012  & 0.021  & 0.025  & 0.051  & 0.049  & 0.033  \\ 
        ~ & Ours$_{\lambda=6.4e-3}$ & 0.015  & 0.063  & 0.044  & 0.013  & 0.022  & 0.027  & 0.071  & 0.055  & 0.039  \\ \midrule
        \multirow{5}{*}{LPIPS$_{VGG}\downarrow$} & DVGO & 0.003  & 0.019  & 0.014  & 0.003  & 0.009  & 0.009  & 0.017  & 0.023  & 0.012  \\ 
        ~ & Ours$_{\lambda=1e-4}$ & 0.003  & 0.020  & 0.014  & 0.003  & 0.009  & 0.010  & 0.017  & 0.023  & 0.013  \\ 
        ~ & Ours$_{\lambda=4e-4}$ & 0.003  & 0.022  & 0.016  & 0.003  & 0.009  & 0.010  & 0.021  & 0.024  & 0.014  \\ 
        ~ & Ours$_{\lambda=1.6e-3}$ & 0.004  & 0.025  & 0.019  & 0.004  & 0.010  & 0.011  & 0.029  & 0.027  & 0.016  \\ 
        ~ & Ours$_{\lambda=6.4e-3}$ & 0.005  & 0.030  & 0.024  & 0.005  & 0.011  & 0.012  & 0.044  & 0.031  & 0.020 \\ 
        \bottomrule
    \end{tabular}
    \caption{Per scene results on Synthetic NSVF dataset with the voxel resolution set to $256^3$~(HR).}
\label{nsvf_hr}
\end{table*}

\begin{table*}[h]
    \centering
    \linespread{1.2} \selectfont
    \begin{tabular}{ccccccc}
        \toprule
        \multicolumn{7}{c}{BlendedMVS} \\
        ~ & Method & Character & Fountain & Jade & Statues & Average  \\ 
        \midrule
        \midrule
        \multirow{5}{*}{SIZE~(MB)$\downarrow$} & DVGO & 136.8  & 73.1  & 163.2  & 104.4  & 119.4  \\ 
        ~ & Ours$_{\lambda=1e-4}$ & 1.593  & 0.870  & 1.829  & 1.378  & 1.418  \\ 
        ~ & Ours$_{\lambda=4e-4}$ & 1.206  & 0.644  & 1.335  & 1.020  & 1.051  \\ 
        ~ & Ours$_{\lambda=1.6e-3}$ & 0.927  & 0.496  & 1.030  & 0.790  & 0.811  \\ 
        ~ & Ours$_{\lambda=6.4e-3}$ & 0.772  & 0.421  & 0.888  & 0.677  & 0.689  \\ \midrule
        \multirow{5}{*}{PSNR~(dB)$\uparrow$} & DVGO & 30.21  & 28.22  & 27.74  & 26.20  & 28.09  \\ 
        ~ & Ours$_{\lambda=1e-4}$ & 30.12  & 28.29  & 27.70  & 26.10  & 28.05  \\ 
        ~ & Ours$_{\lambda=4e-4}$ & 29.96  & 28.07  & 27.67  & 26.08  & 27.94  \\ 
        ~ & Ours$_{\lambda=1.6e-3}$ & 29.52  & 27.56  & 27.53  & 25.99  & 27.65  \\ 
        ~ & Ours$_{\lambda=6.4e-3}$ & 28.75  & 26.78  & 27.24  & 25.75  & 27.13  \\ \midrule
        \multirow{5}{*}{SSIM$\uparrow$} & DVGO & 0.963  & 0.923  & 0.916  & 0.886  & 0.922  \\ 
        ~ & Ours$_{\lambda=1e-4}$ & 0.961  & 0.920  & 0.915  & 0.881  & 0.919  \\ 
        ~ & Ours$_{\lambda=4e-4}$ & 0.959  & 0.912  & 0.911  & 0.878  & 0.915  \\ 
        ~ & Ours$_{\lambda=1.6e-3}$ & 0.954  & 0.895  & 0.903  & 0.868  & 0.905  \\ 
        ~ & Ours$_{\lambda=6.4e-3}$ & 0.944  & 0.871  & 0.892  & 0.855  & 0.890  \\ \midrule
        \multirow{5}{*}{LPIPS$_{ALEX}\downarrow$} & DVGO & 0.046  & 0.117  & 0.105  & 0.136  & 0.101  \\ 
        ~ & Ours$_{\lambda=1e-4}$ & 0.048  & 0.120  & 0.107  & 0.140  & 0.104  \\ 
        ~ & Ours$_{\lambda=4e-4}$ & 0.051  & 0.129  & 0.113  & 0.146  & 0.110  \\ 
        ~ & Ours$_{\lambda=1.6e-3}$ & 0.057  & 0.146  & 0.124  & 0.156  & 0.120  \\ 
        ~ & Ours$_{\lambda=6.4e-3}$ & 0.066  & 0.165  & 0.135  & 0.169  & 0.133  \\ \midrule
        \multirow{5}{*}{LPIPS$_{VGG}\downarrow$} & DVGO & 0.029  & 0.085  & 0.072  & 0.107  & 0.073  \\ 
        ~ & Ours$_{\lambda=1e-4}$ & 0.029  & 0.087  & 0.073  & 0.110  & 0.075  \\ 
        ~ & Ours$_{\lambda=4e-4}$ & 0.031  & 0.095  & 0.077  & 0.118  & 0.080  \\ 
        ~ & Ours$_{\lambda=1.6e-3}$ & 0.036  & 0.110  & 0.085  & 0.131  & 0.090  \\ 
        ~ & Ours$_{\lambda=6.4e-3}$ & 0.045  & 0.131  & 0.094  & 0.143  & 0.103 \\ 
        \bottomrule
    \end{tabular}
    \caption{Per scene results on BlendedMVS dataset with the voxel resolution set to $160^3$.}
\label{mvs_base}
\end{table*}

\setlength{\tabcolsep}{5pt} % Adjust horizontal spacing
\begin{table*}[h]
    \centering
    \linespread{1.2} \selectfont
    \begin{tabular}{ccccccc}
        \toprule
        \multicolumn{7}{c}{BlendedMVS~(HR)} \\
        ~ & Method & Character & Fountain & Jade & Statues & Average  \\ 
        \midrule
        \midrule
        \multirow{5}{*}{SIZE~(MB)$\downarrow$} & DVGO & 509.1  & 252.3  & 638.8  & 375.1  & 443.8  \\ 
        ~ & Ours$_{\lambda=1e-4}$ & 4.971  & 2.800  & 6.515  & 5.064  & 4.837  \\ 
        ~ & Ours$_{\lambda=4e-4}$ & 3.810  & 2.090  & 4.874  & 3.783  & 3.639  \\ 
        ~ & Ours$_{\lambda=1.6e-3}$ & 2.911  & 1.588  & 3.716  & 2.856  & 2.768  \\ 
        ~ & Ours$_{\lambda=6.4e-3}$ & 2.393  & 1.324  & 3.126  & 2.375  & 2.304  \\ \midrule
        \multirow{5}{*}{PSNR~(dB)$\uparrow$} & DVGO & 30.91  & 29.43  & 27.67  & 26.37  & 28.59  \\ 
        ~ & Ours$_{\lambda=1e-4}$ & 30.85  & 29.48  & 27.59  & 26.28  & 28.55  \\ 
        ~ & Ours$_{\lambda=4e-4}$ & 30.80  & 29.37  & 27.59  & 26.30  & 28.52  \\ 
        ~ & Ours$_{\lambda=1.6e-3}$ & 30.61  & 29.07  & 27.55  & 26.32  & 28.39  \\ 
        ~ & Ours$_{\lambda=6.4e-3}$ & 30.12  & 28.47  & 27.43  & 26.22  & 28.06  \\ \midrule
        \multirow{5}{*}{SSIM$\uparrow$} & DVGO & 0.970  & 0.942  & 0.920  & 0.899  & 0.933  \\ 
        ~ & Ours$_{\lambda=1e-4}$ & 0.969  & 0.941  & 0.918  & 0.896  & 0.931  \\ 
        ~ & Ours$_{\lambda=4e-4}$ & 0.969  & 0.938  & 0.917  & 0.896  & 0.930  \\ 
        ~ & Ours$_{\lambda=1.6e-3}$ & 0.966  & 0.929  & 0.914  & 0.891  & 0.925  \\ 
        ~ & Ours$_{\lambda=6.4e-3}$ & 0.961  & 0.913  & 0.907  & 0.881  & 0.915  \\ \midrule
        \multirow{5}{*}{LPIPS$_{ALEX}\downarrow$} & DVGO & 0.037  & 0.088  & 0.092  & 0.111  & 0.082  \\ 
        ~ & Ours$_{\lambda=1e-4}$ & 0.038  & 0.088  & 0.093  & 0.113  & 0.083  \\ 
        ~ & Ours$_{\lambda=4e-4}$ & 0.039  & 0.094  & 0.095  & 0.116  & 0.086  \\ 
        ~ & Ours$_{\lambda=1.6e-3}$ & 0.042  & 0.105  & 0.101  & 0.123  & 0.093  \\ 
        ~ & Ours$_{\lambda=6.4e-3}$ & 0.048  & 0.120  & 0.110  & 0.134  & 0.103  \\ \midrule
        \multirow{5}{*}{LPIPS$_{VGG}\downarrow$} & DVGO & 0.021  & 0.054  & 0.058  & 0.075  & 0.052  \\ 
        ~ & Ours$_{\lambda=1e-4}$ & 0.021  & 0.052  & 0.057  & 0.075  & 0.051  \\ 
        ~ & Ours$_{\lambda=4e-4}$ & 0.022  & 0.057  & 0.059  & 0.078  & 0.054  \\ 
        ~ & Ours$_{\lambda=1.6e-3}$ & 0.023  & 0.067  & 0.063  & 0.086  & 0.060  \\ 
        ~ & Ours$_{\lambda=6.4e-3}$ & 0.027  & 0.081  & 0.069  & 0.097  & 0.069 \\ 
        \bottomrule
    \end{tabular}
    \caption{Per scene results on BlendedMVS dataset with the voxel resolution set to $256^3$~(HR).}
\label{mvs_hr}
\end{table*}

\begin{table*}[h]
    \centering
    \linespread{1.2} \selectfont
    \begin{tabular}{cccccccc}
        \toprule
        \multicolumn{8}{c}{Tanks \& Temples} \\
        ~ & Method & Barn & Caterpillar & Family & Ignatius & Truck & Average \\
        \midrule
        \midrule
        \multirow{5}{*}{SIZE~(MB)$\downarrow$} & DVGO & 142.3  & 116.5  & 97.5  & 97.4  & 112.5  & 113.2  \\ 
        ~ & Ours$_{\lambda=1e-4}$ & 1.889  & 1.320  & 1.064  & 0.859  & 1.425  & 1.311  \\ 
        ~ & Ours$_{\lambda=4e-4}$ & 1.414  & 0.990  & 0.814  & 0.641  & 1.071  & 0.986  \\ 
        ~ & Ours$_{\lambda=1.6e-3}$ & 1.109  & 0.771  & 0.653  & 0.514  & 0.830  & 0.775  \\ 
        ~ & Ours$_{\lambda=6.4e-3}$ & 0.952  & 0.659  & 0.571  & 0.456  & 0.704  & 0.668  \\ \midrule
        \multirow{5}{*}{PSNR~(dB)$\uparrow$} & DVGO & 26.86  & 25.80  & 33.69  & 27.91  & 27.08  & 28.27  \\ 
        ~ & Ours$_{\lambda=1e-4}$ & 26.80  & 25.81  & 33.69  & 27.77  & 27.09  & 28.23  \\ 
        ~ & Ours$_{\lambda=4e-4}$ & 26.73  & 25.72  & 33.49  & 27.80  & 27.02  & 28.15  \\ 
        ~ & Ours$_{\lambda=1.6e-3}$ & 26.56  & 25.52  & 33.06  & 27.70  & 26.80  & 27.93  \\ 
        ~ & Ours$_{\lambda=6.4e-3}$ & 26.18  & 25.20  & 32.34  & 27.47  & 26.41  & 27.52  \\ \midrule
        \multirow{5}{*}{SSIM$\uparrow$} & DVGO & 0.839  & 0.905  & 0.962  & 0.940  & 0.905  & 0.910  \\ 
        ~ & Ours$_{\lambda=1e-4}$ & 0.839  & 0.904  & 0.961  & 0.939  & 0.905  & 0.909  \\ 
        ~ & Ours$_{\lambda=4e-4}$ & 0.836  & 0.902  & 0.958  & 0.938  & 0.902  & 0.907  \\ 
        ~ & Ours$_{\lambda=1.6e-3}$ & 0.831  & 0.897  & 0.954  & 0.935  & 0.896  & 0.903  \\ 
        ~ & Ours$_{\lambda=6.4e-3}$ & 0.820  & 0.891  & 0.947  & 0.932  & 0.888  & 0.896  \\ \midrule
        \multirow{5}{*}{LPIPS$_{ALEX}\downarrow$} & DVGO & 0.294  & 0.169  & 0.070  & 0.090  & 0.161  & 0.157  \\ 
        ~ & Ours$_{\lambda=1e-4}$ & 0.295  & 0.173  & 0.073  & 0.092  & 0.163  & 0.159  \\ 
        ~ & Ours$_{\lambda=4e-4}$ & 0.301  & 0.177  & 0.077  & 0.094  & 0.168  & 0.163  \\ 
        ~ & Ours$_{\lambda=1.6e-3}$ & 0.311  & 0.183  & 0.082  & 0.097  & 0.176  & 0.170  \\ 
        ~ & Ours$_{\lambda=6.4e-3}$ & 0.327  & 0.192  & 0.090  & 0.101  & 0.187  & 0.179  \\ \midrule
        \multirow{5}{*}{LPIPS$_{VGG}\downarrow$} & DVGO & 0.288  & 0.151  & 0.063  & 0.095  & 0.147  & 0.149  \\ 
        ~ & Ours$_{\lambda=1e-4}$ & 0.285  & 0.154  & 0.064  & 0.099  & 0.146  & 0.150  \\ 
        ~ & Ours$_{\lambda=4e-4}$ & 0.293  & 0.159  & 0.068  & 0.101  & 0.151  & 0.154  \\ 
        ~ & Ours$_{\lambda=1.6e-3}$ & 0.308  & 0.168  & 0.072  & 0.105  & 0.160  & 0.163  \\ 
        ~ & Ours$_{\lambda=6.4e-3}$ & 0.336  & 0.181  & 0.079  & 0.109  & 0.173  & 0.176 \\ 
        \bottomrule
    \end{tabular}
    \caption{Per scene results on Tanks \& Temples dataset with the voxel resolution set to $160^3$.}
\label{tnt}
\end{table*}

\begin{table*}[h]
    \centering
    \linespread{1.2} \selectfont
    \begin{tabular}{cccccccc}
        \toprule
        \multicolumn{8}{c}{Tanks \& Temples~(HR)} \\
        ~ & Method & Barn & Caterpillar & Family & Ignatius & Truck & Average \\
        \midrule
        \midrule
        \multirow{5}{*}{SIZE~(MB)$\downarrow$} & DVGO & 525.7  & 427.4  & 360.0  & 354.2  & 419.7  & 417.4  \\ 
        ~ & Ours$_{\lambda=1e-4}$ & 5.825  & 4.536  & 3.851  & 2.698  & 4.733  & 4.329  \\ 
        ~ & Ours$_{\lambda=4e-4}$ & 4.455  & 3.442  & 2.969  & 2.008  & 3.599  & 3.295  \\ 
        ~ & Ours$_{\lambda=1.6e-3}$ & 3.435  & 2.647  & 2.351  & 1.570  & 2.746  & 2.550  \\ 
        ~ & Ours$_{\lambda=6.4e-3}$ & 2.860  & 2.212  & 2.013  & 1.354  & 2.272  & 2.142  \\ \midrule
        \multirow{5}{*}{PSNR~(dB)$\uparrow$} & DVGO & 27.34  & 26.11  & 34.24  & 28.13  & 27.45  & 28.66  \\ 
        ~ & Ours$_{\lambda=1e-4}$ & 27.36  & 26.17  & 34.31  & 28.06  & 27.50  & 28.68  \\ 
        ~ & Ours$_{\lambda=4e-4}$ & 27.30  & 26.14  & 34.23  & 28.04  & 27.46  & 28.63  \\ 
        ~ & Ours$_{\lambda=1.6e-3}$ & 27.20  & 26.07  & 34.00  & 27.97  & 27.37  & 28.52  \\ 
        ~ & Ours$_{\lambda=6.4e-3}$ & 26.98  & 25.92  & 33.54  & 27.86  & 27.15  & 28.29  \\ \midrule
        \multirow{5}{*}{SSIM$\uparrow$} & DVGO & 0.857  & 0.912  & 0.967  & 0.945  & 0.917  & 0.920  \\ 
        ~ & Ours$_{\lambda=1e-4}$ & 0.859  & 0.912  & 0.967  & 0.945  & 0.917  & 0.920  \\ 
        ~ & Ours$_{\lambda=4e-4}$ & 0.857  & 0.911  & 0.966  & 0.944  & 0.915  & 0.919  \\ 
        ~ & Ours$_{\lambda=1.6e-3}$ & 0.853  & 0.909  & 0.963  & 0.942  & 0.912  & 0.916  \\ 
        ~ & Ours$_{\lambda=6.4e-3}$ & 0.845  & 0.905  & 0.958  & 0.938  & 0.904  & 0.910  \\ \midrule
        \multirow{5}{*}{LPIPS$_{ALEX}\downarrow$} & DVGO & 0.264  & 0.155  & 0.059  & 0.082  & 0.142  & 0.141  \\ 
        ~ & Ours$_{\lambda=1e-4}$ & 0.262  & 0.156  & 0.060  & 0.083  & 0.142  & 0.140  \\ 
        ~ & Ours$_{\lambda=4e-4}$ & 0.266  & 0.158  & 0.063  & 0.085  & 0.145  & 0.144  \\ 
        ~ & Ours$_{\lambda=1.6e-3}$ & 0.275  & 0.163  & 0.068  & 0.088  & 0.152  & 0.149  \\ 
        ~ & Ours$_{\lambda=6.4e-3}$ & 0.288  & 0.170  & 0.074  & 0.092  & 0.161  & 0.157  \\ \midrule
        \multirow{5}{*}{LPIPS$_{VGG}\downarrow$} & DVGO & 0.243  & 0.132  & 0.052  & 0.083  & 0.124  & 0.127  \\ 
        ~ & Ours$_{\lambda=1e-4}$ & 0.236  & 0.131  & 0.052  & 0.084  & 0.122  & 0.125  \\ 
        ~ & Ours$_{\lambda=4e-4}$ & 0.240  & 0.134  & 0.054  & 0.086  & 0.124  & 0.128  \\ 
        ~ & Ours$_{\lambda=1.6e-3}$ & 0.251  & 0.139  & 0.058  & 0.088  & 0.130  & 0.133  \\ 
        ~ & Ours$_{\lambda=6.4e-3}$ & 0.270  & 0.147  & 0.062  & 0.093  & 0.139  & 0.142 \\ 
        \bottomrule
    \end{tabular}
    \caption{Per scene results on Tanks \& Temples dataset with the voxel resolution set to $256^3$~(HR).}
\label{tnt_hr}
\end{table*}
